# Supplementary material for: BachVid: Training-Free Video Generation with Consistent Background and Character
Source: arXiv:2510.21696 source file (2025-10-24)
Supplement: Supplementary file 1 [file appendix.tex]

\section{Usage of LLM}
We use ChatGPT to polish our writing, and use DeepSeek for text-to-video prompt generation, which is used as evaluation dataset.
